# Supplementary material for: Smartphone Impostor Detection with Built-in Sensors and Deep Learning
Source: arXiv:2002.03914 source file (2020-02-10)
Supplement: Supplementary file 1 [file appendix0201_SwMetrics.tex]

\section{Metrics of Accuracy}
\label{apd_sw_metric}

The true negative rate (TNR) is defined as $TNR = \frac{TN}{\vert N\vert} = \frac{TN}{TN+FP}$ %in~\gyrefeq{eq_tnr} 
where $\vert N\vert$ is the number of samples from the real user, which can be further divided into the true negatives (TN) and the false positives (FP). %TN is the number of samples from the correct user which do not get rejected while FP is the number of samples from the correct user which are erroneously recognized as an impostor and rejected. 
A low TNR means that very few users will tend to enable the detection mechanism (low usability).
\iffalse
\begin{equation}
\begin{split}
  &TNR = \frac{TN}{\vert N\vert} = \frac{TN}{TN+FP} \\
\end{split}
\label{eq_tnr}
\end{equation}
\fi

The true positive rate (TPR) is defined as $TPR = \frac{TP}{\vert P\vert} = \frac{TP}{TP+FN}$ %in \gyrefeq{eq_tpr} 
where $\vert P\vert$ is the total number of samples from an impostor which is the sum of the true positive number (TP) and the false negative number (FN). %TP counts the samples from the impostor which are successfully rejected while FN counts the other samples from the impostor that pass the detection and are not rejected. 
A detection mechanism has little security if its TPR is low.
\iffalse
\begin{equation}
\begin{split}
  &TPR = \frac{TP}{\vert P\vert} = \frac{TP}{TP+FN} \\
\end{split}
\label{eq_tpr}
\end{equation}
\fi

The average accuracy is computed for all the testing samples including the real user and an impostor. When the dataset is balanced, the accuracy is equal to the average of TNR and TPR (see ~\gyrefeq{eq_rpf}). Other three metrics, recall (R), precision (P) and F1 score, are also defined in~\gyrefeq{eq_rpf}. 
\iffalse
\begin{equation}
\begin{split}
  
\end{split}
%\label{eq_tpr}
\end{equation}
\fi
\begin{equation}
\begin{split}
  Accuracy &= \frac{TN+TP}{\vert N\vert+\vert P\vert}
  %\stackrel{
  %\begin{split}
  % &\text{balanced} \\
  % &\textnormal{~dataset}
  %\end{split}
  %\parbox{0.7cm}{balanced\\~~dataset\\}
  %}{=} 
  \approx \frac{TNR+TPR}{2} (if~\vert N\vert \approx \vert P\vert)\\
  Recall &= TPR \\
  Precision &= \frac{TP}{TP+FP} = \frac{\vert P\vert\times TPR}{\vert P\vert\times TPR+\vert N\vert \times FPR}\\
  %&\approx \frac{TPR}{TPR+1-TNR}(if~\vert N\vert \approx \vert P\vert) \\
  F1 score &= \frac{2 \times Recall \times Precision}{Recall+Precision}
\end{split}
\label{eq_rpf}
\end{equation}
