# Supplementary material for: Smartphone Impostor Detection with Built-in Sensors and Deep Learning
Source: arXiv:2002.03914 source file (2020-02-10)
Supplement: Supplementary file 2 [file appendix0301_pseudocode.tex]

\section{Pseudo-codes in \modulename}
\label{apd_pseudo_code}
